# Supplementary material for: GPT-4V-AD: Exploring Grounding Potential of VQA-oriented GPT-4V for Zero-shot Anomaly Detection
Source: arXiv:2311.02612 source file (2024-04-16)
Supplement: Supplementary file 1 [file 6_appendix.tex]

\appendix
